# Supplementary material for: Phase transitions in inorganic halide perovskites from machine learning potentials
Source: arXiv:2301.03497 ancillary file (2023-01-09)
Supplement: Supplementary file 1 [file sm.pdf]

## **Supplemental Material:**

### **Phase transitions in inorganic halide perovskites from machine learning potentials**

Erik Fransson, Julia Wiktor, and Paul Erhart

*Department of Physics, Chalmers University of Technology, SE-41296, Gothenburg, Sweden*

## **Contents**

|                                |           |
|--------------------------------|-----------|
| <b>Supplemental Figures</b>    | <b>2</b>  |
| <b>Supplemental Tables</b>     | <b>9</b>  |
| <b>Supplemental References</b> | <b>14</b> |

## Supplemental Figures

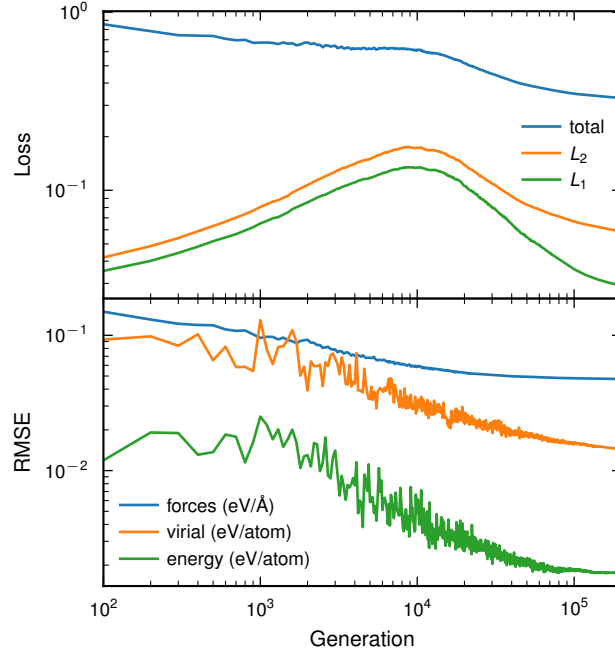

Figure S1: Evolution of total loss as well as its individual contributions during training of the full model for  $\text{CsPbI}_3$  based on the vdW-DF-cx functional.  $L_1$ ,  $L_2$ : contribution from  $L_1/L_2$ -norm of parameter vector. See Ref. 1 for full definition of loss function.

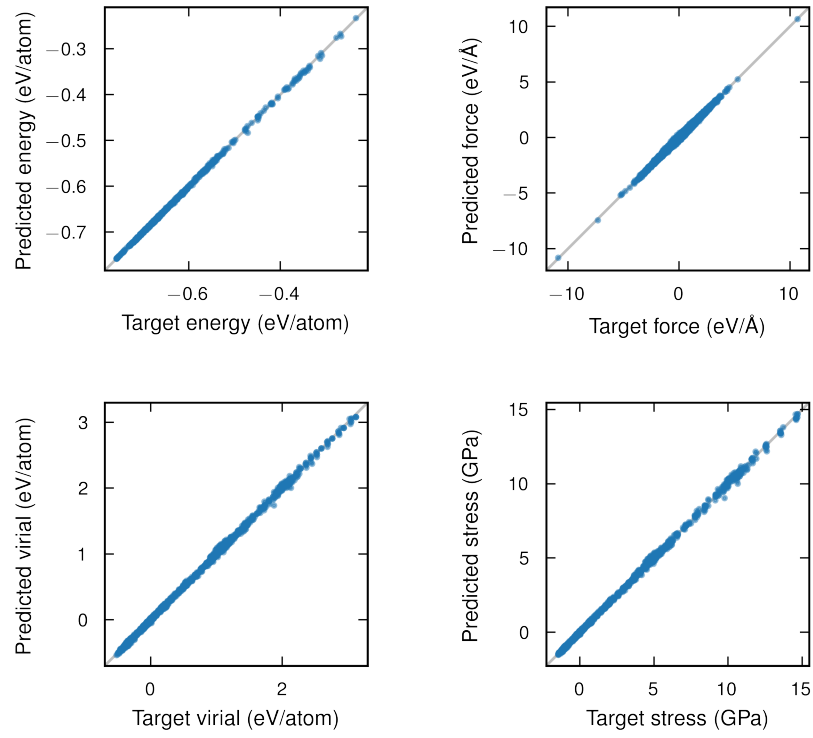

Figure S2: Parity plots for the full model for  $\text{CsPbI}_3$  based on the vdW-DF-cx functional.

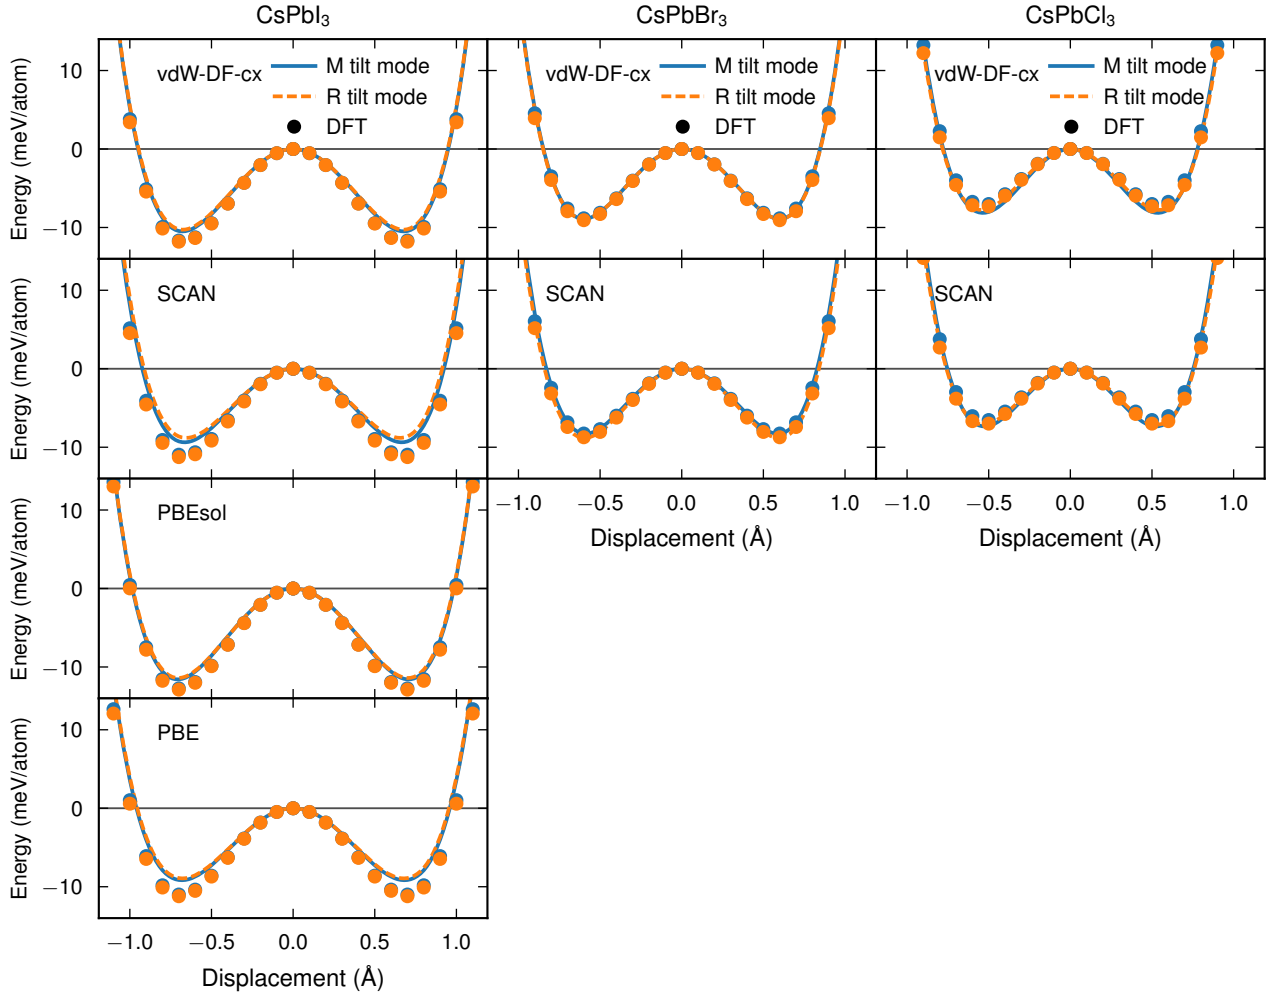

Figure S3: Potential energy landscapes along the in-phase M tilt mode and the out-of-plane R tilt mode for all systems with different functionals. The  $x$ -axis indicates the atomic displacement of an X atom (X=I, Br, Cl) involved in the tilt motion.

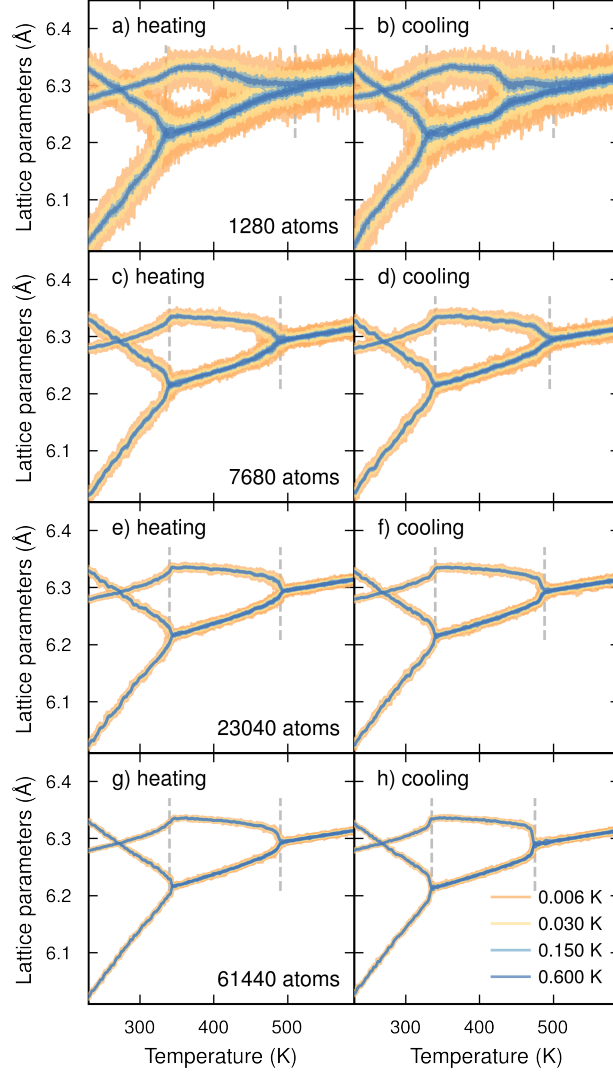

Figure S4: Effect of Hamming window size on lattice parameter data for different supercell sizes at a heating/cooling rate of  $R = 6 \text{ K/ns}$ . The Hamming window  $w_T$  is given in temperature units which is related to the window size in time units  $w_t$  as  $w_T = R w_t$ . Data from full model for  $\text{CsPbI}_3$  based on the vdW-DF-cx functional.

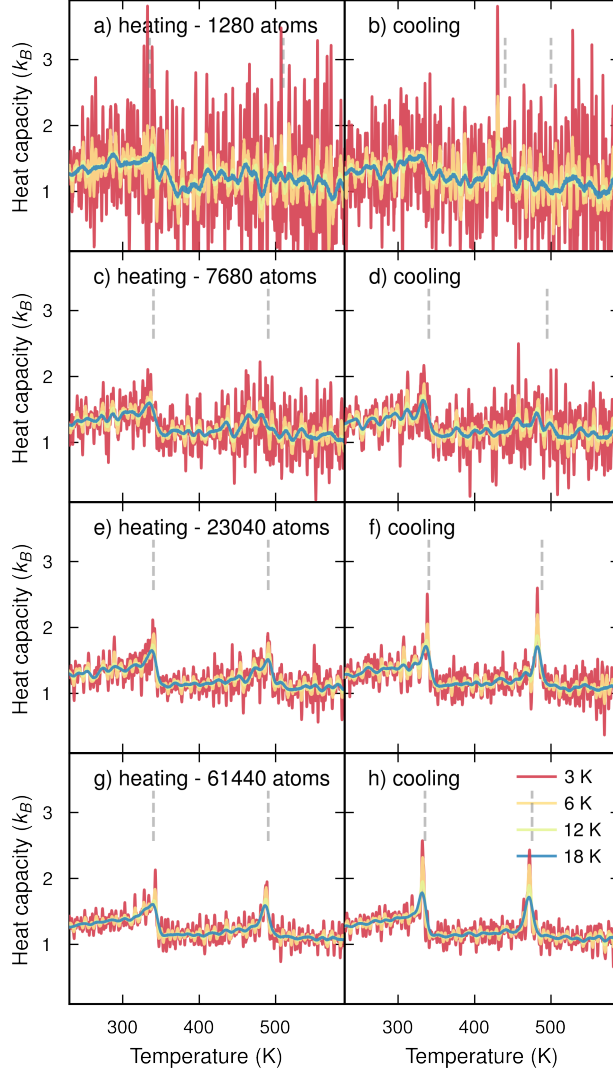

Figure S5: Effect of Hamming window size on heat capacity data for different supercell sizes at a heating/cooling rate of  $R = 6 \text{ K/ns}$ . The Hamming window  $w_T$  is given in temperature units which is related to the window size in time units  $w_t$  as  $w_T = R w_t$ . Data from full model for  $\text{CsPbI}_3$  based on the vdW-DF-cx functional.

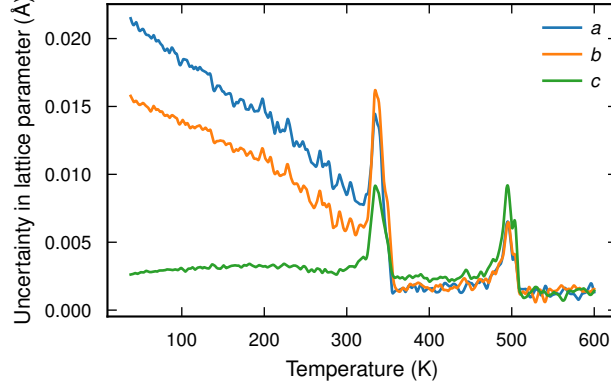

Figure S6: Uncertainty in predictions of the lattice parameters. The uncertainty is estimated as the standard deviation over the predictions from the five models included in the model ensemble. Data from full model for  $\text{CsPbI}_3$  based on the vdW-DF-cx functional.

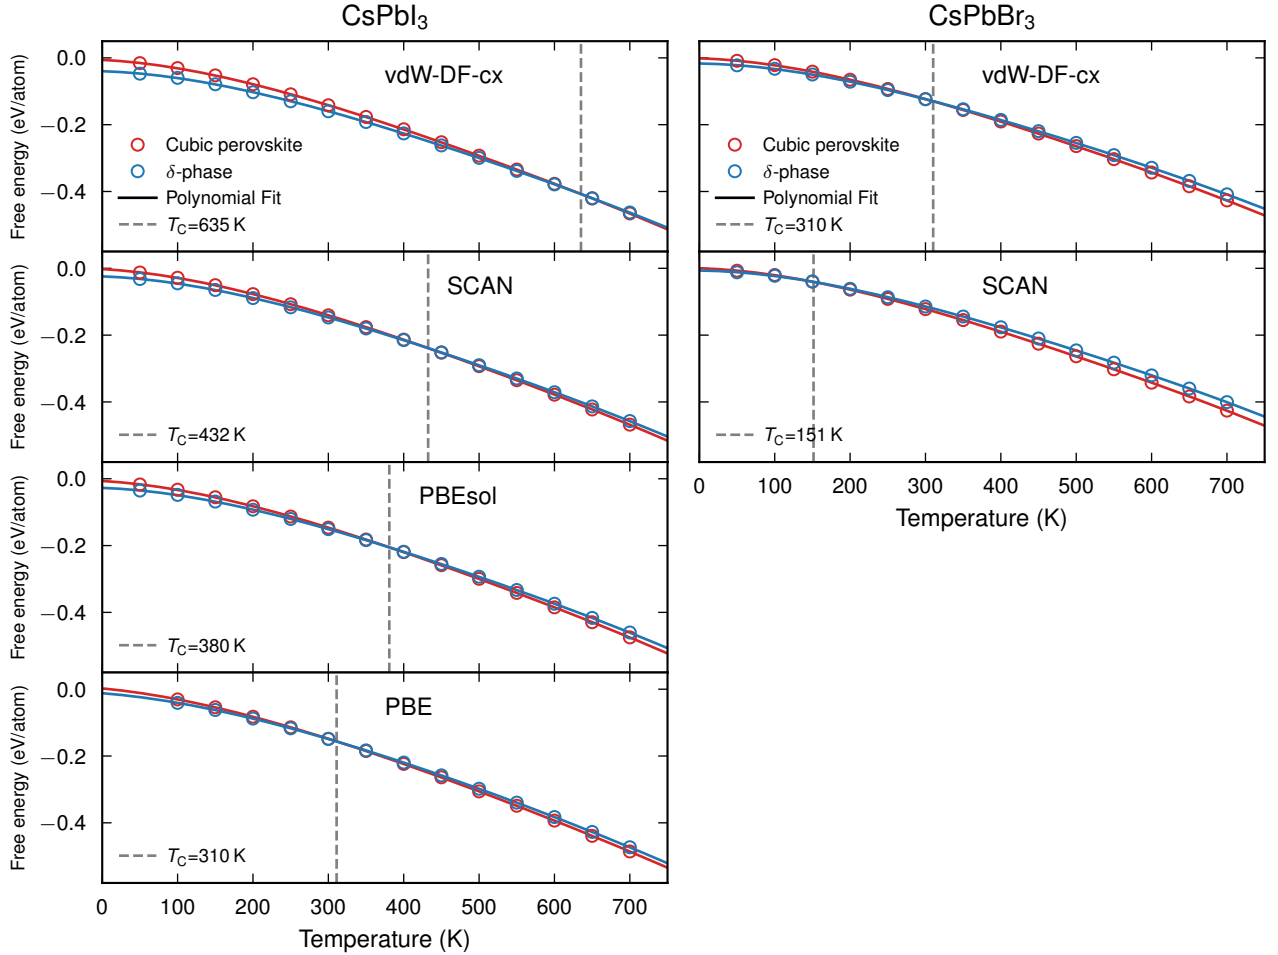

Figure S7: Free energies of the  $\delta$  and cubic perovskite phases from thermodynamic integration. The crossing between the two landscapes yields the transition temperatures reported in Table II of the main manuscript. In these simulations, the perovskite structure was constrained to have the cubic lattice constants corresponding to the respective temperature. Distortions of the cell metric were thus constrained but the atomic displacements were fully sampled.

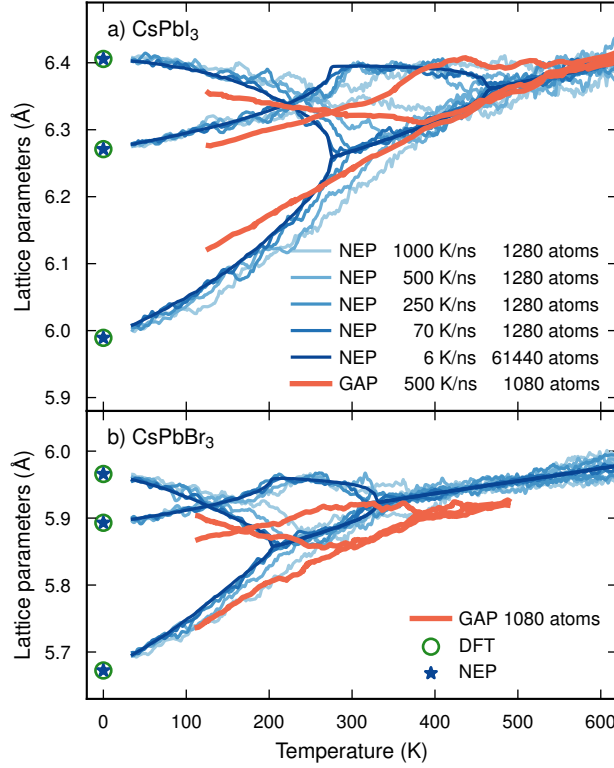

Figure S8: Lattice parameters as a function of temperature for (a)  $\text{CsPbI}_3$  and (b)  $\text{CsPbBr}_3$  from NEP (“full” models) and GAP models based on the SCAN XC functional. The results from the latter were taken from Refs. 2 and 3. The heating/cooling rate for the  $\text{CsPbBr}_3$  run from Ref. 3 is not explicitly stated but is expected to be comparable to the one used for  $\text{CsPbI}_3$  in Ref. 2. The results show that the use of high rates and small cells can lead to a considerable overestimation of the transition temperatures on heating by as much as 100 K. Also note that the NEP results smoothly extrapolate to the lattice parameters obtained in the static (0 K) limit, in which NEP and DFT data match very closely (also see Table S4 below). In the NEP simulations we used supercells comprising  $4 \times 4 \times 4$  primitive orthorhombic cells corresponding to 1280 atoms. The data were subjected to a Hamming filter with a window of 5 K or less to smoothen the data.

# Supplemental Tables

Table S1: RMSE scores (first rows) and coefficient of determination ( $R^2$ ; second rows) for the final NEP models obtained by training against the full data set (“full”) and the respective model ensemble (“ensemble”). the RMSE scores are given in units of meV/atom for energies and virials and in units of meV/Å for the forces. The “Structures” column specifies the number of structures (first rows) and the number of force components (second rows) used during training of the individual models.

|                     | Structures |          | Energies |              | Forces |              | Virials |              |
|---------------------|------------|----------|----------|--------------|--------|--------------|---------|--------------|
|                     | full       | ensemble | full     | ensemble     | full   | ensemble     | full    | ensemble     |
| CsPbBr <sub>3</sub> |            |          |          |              |        |              |         |              |
| vdW-DF-cx           | 618        | 556      | 1.1      | 1.1 + 0.0    | 45.1   | 45.0 + 0.3   | 11.1    | 11.4 + 0.6   |
|                     | 189 765    | 170 451  | 0.9999   | 0.9999 + 0.0 | 0.9868 | 0.9868 + 0.0 | 0.9997  | 0.9997 + 0.0 |
| SCAN                | 617        | 555      | 1.2      | 1.4 + 0.2    | 47.6   | 48.0 + 0.2   | 15.1    | 13.7 + 0.5   |
|                     | 188 790    | 169 422  | 0.9999   | 0.9998 + 0.0 | 0.9853 | 0.9851 + 0.0 | 0.9995  | 0.9996 + 0.0 |
| CsPbCl <sub>3</sub> |            |          |          |              |        |              |         |              |
| vdW-DF-cx           | 633        | 569      | 1.2      | 1.1 + 0.1    | 46.4   | 45.7 + 0.3   | 13.0    | 12.7 + 0.4   |
|                     | 197 460    | 177 705  | 0.9998   | 0.9999 + 0.0 | 0.9883 | 0.9888 + 0.0 | 0.9996  | 0.9996 + 0.0 |
| SCAN                | 617        | 555      | 1.1      | 1.2 + 0.1    | 47.8   | 47.9 + 0.3   | 14.0    | 15.3 + 0.8   |
|                     | 189 435    | 170 220  | 0.9999   | 0.9999 + 0.0 | 0.9871 | 0.9871 + 0.0 | 0.9996  | 0.9995 + 0.0 |
| CsPbI <sub>3</sub>  |            |          |          |              |        |              |         |              |
| vdW-DF-cx           | 674        | 606      | 1.8      | 1.7 + 0.1    | 47.5   | 47.5 + 0.2   | 14.5    | 14.9 + 1.0   |
|                     | 195 180    | 174 816  | 0.9997   | 0.9997 + 0.0 | 0.9862 | 0.9862 + 0.0 | 0.9994  | 0.9994 + 0.0 |
| SCAN                | 657        | 591      | 2.1      | 2.2 + 0.0    | 51.4   | 51.6 + 0.4   | 16.0    | 16.6 + 0.4   |
|                     | 184 080    | 165 324  | 0.9998   | 0.9998 + 0.0 | 0.9871 | 0.9869 + 0.0 | 0.9996  | 0.9996 + 0.0 |
| PBEsol              | 697        | 627      | 1.9      | 1.8 + 0.1    | 50.6   | 50.1 + 0.2   | 15.2    | 14.4 + 0.9   |
|                     | 208 020    | 186 429  | 0.9997   | 0.9998 + 0.0 | 0.9909 | 0.9911 + 0.0 | 0.9995  | 0.9996 + 0.0 |
| PBE                 | 510        | 459      | 1.0      | 1.2 + 0.1    | 43.1   | 43.2 + 0.3   | 12.6    | 13.8 + 1.3   |
|                     | 137 400    | 122 838  | 0.9999   | 0.9999 + 0.0 | 0.9862 | 0.9861 + 0.0 | 0.9996  | 0.9995 + 0.0 |

Table S2: Comparison of energy differences  $\Delta E$  for  $\text{CsPbCl}_3$  structures relative to the orthorhombic phase in meV/atom and lattice parameters  $a$ ,  $b$ , and  $c$  in Å from density functional theory (DFT) calculations as well as the neuroevolution potential (NEP) models constructed in this work. For the latter results are given both for the models trained against the full set and model ensembles. In the latter case, the uncertainty obtained as the standard deviation across the models in the ensemble is given as well.

| CsPbCl <sub>3</sub>                              | vdW-DF-cx |            |                    | SCAN   |            |                    |
|--------------------------------------------------|-----------|------------|--------------------|--------|------------|--------------------|
|                                                  | DFT       | NEP (full) | NEP (ensemble)     | DFT    | NEP (full) | NEP (ensemble)     |
| orthorhombic ( $Pnma$ , $a^-a^-c^+$ )            |           |            |                    |        |            |                    |
| $a$                                              | 7.683     | 7.683      | $7.672 \pm 0.042$  | 7.692  | 7.694      | $7.709 \pm 0.011$  |
| $b$                                              | 8.034     | 8.034      | $8.044 \pm 0.023$  | 8.054  | 8.067      | $8.056 \pm 0.011$  |
| $c$                                              | 11.227    | 11.227     | $11.238 \pm 0.014$ | 11.257 | 11.268     | $11.265 \pm 0.003$ |
| tetragonal perovskite ( $P4/mbm$ , $a^0a^0c^+$ ) |           |            |                    |        |            |                    |
| $\Delta E$                                       | 2.8       | 3.2        | $2.6 \pm 0.3$      | 2.5    | 3.0        | $2.8 \pm 0.1$      |
| $a$                                              | 7.803     | 7.803      | $7.806 \pm 0.004$  | 7.831  | 7.831      | $7.831 \pm 0.002$  |
| $b$                                              | 7.803     | 7.803      | $7.806 \pm 0.004$  | 7.831  | 7.831      | $7.831 \pm 0.002$  |
| $c$                                              | 5.699     | 5.699      | $5.699 \pm 0.003$  | 5.705  | 5.705      | $5.704 \pm 0.002$  |
| tetragonal perovskite ( $I4/mcm$ , $a^0a^0c^-$ ) |           |            |                    |        |            |                    |
| $\Delta E$                                       | 2.5       | 3.6        | $2.8 \pm 0.1$      | 1.9    | 3.2        | $2.9 \pm 0.4$      |
| $a$                                              | 7.803     | 7.803      | $7.806 \pm 0.004$  | 7.829  | 7.829      | $7.829 \pm 0.002$  |
| $b$                                              | 7.803     | 7.803      | $7.806 \pm 0.004$  | 7.829  | 7.829      | $7.829 \pm 0.002$  |
| $c$                                              | 11.401    | 11.401     | $11.399 \pm 0.004$ | 11.415 | 11.415     | $11.409 \pm 0.005$ |
| cubic perovskite ( $Pm\bar{3}m$ , $a^0a^0a^0$ )  |           |            |                    |        |            |                    |
| $\Delta E$                                       | 14.0      | 15.8       | $14.7 \pm 0.6$     | 12.5   | 14.0       | $13.6 \pm 0.4$     |
| $a$                                              | 5.636     | 5.636      | $5.633 \pm 0.002$  | 5.640  | 5.640      | $5.640 \pm 0.001$  |
| $b$                                              | 5.636     | 5.636      | $5.633 \pm 0.002$  | 5.640  | 5.640      | $5.640 \pm 0.001$  |
| $c$                                              | 5.636     | 5.636      | $5.633 \pm 0.002$  | 5.640  | 5.640      | $5.640 \pm 0.001$  |
| $\delta$ -phase ( $Pnma$ )                       |           |            |                    |        |            |                    |
| $\Delta E$                                       | -0.3      | -0.5       | $-0.5 \pm 0.1$     | 6.8    | 7.2        | $7.0 \pm 0.2$      |
| $a$                                              | 9.164     | 4.432      | $4.416 \pm 0.005$  | 4.429  | 4.429      | $4.438 \pm 0.005$  |
| $b$                                              | 4.432     | 9.164      | $9.167 \pm 0.011$  | 9.237  | 9.237      | $9.228 \pm 0.017$  |
| $c$                                              | 16.003    | 16.003     | $16.056 \pm 0.016$ | 16.204 | 16.204     | $16.205 \pm 0.023$ |

Table S3: Comparison of energy differences  $\Delta E$  for CsPbBr<sub>3</sub> structures relative to the orthorhombic phase in meV/atom and lattice parameters  $a$ ,  $b$ , and  $c$  in Å from density functional theory (DFT) calculations as well as the neuroevolution potential (NEP) models constructed in this work. For the latter results are given both for the models trained against the full set and model ensembles. In the latter case, the uncertainty obtained as the standard deviation across the models in the ensemble is given as well.

| CsPbBr <sub>3</sub>                              | vdW-DF-cx |            |                    | SCAN   |            |                    |
|--------------------------------------------------|-----------|------------|--------------------|--------|------------|--------------------|
|                                                  | DFT       | NEP (full) | NEP (ensemble)     | DFT    | NEP (full) | NEP (ensemble)     |
| orthorhombic ( $Pnma$ , $a^-a^-c^+$ )            |           |            |                    |        |            |                    |
| $a$                                              | 7.906     | 7.906      | $7.881 \pm 0.021$  | 8.022  | 8.022      | $7.996 \pm 0.012$  |
| $b$                                              | 8.438     | 8.438      | $8.469 \pm 0.013$  | 8.437  | 8.437      | $8.450 \pm 0.011$  |
| $c$                                              | 11.742    | 11.742     | $11.740 \pm 0.011$ | 11.786 | 11.786     | $11.785 \pm 0.023$ |
| tetragonal perovskite ( $P4/mbm$ , $a^0a^0c^+$ ) |           |            |                    |        |            |                    |
| $\Delta E$                                       | 4.5       | 3.9        | $4.4 \pm 0.5$      | 3.8    | 3.3        | $3.9 \pm 0.4$      |
| $a$                                              | 8.144     | 8.144      | $8.152 \pm 0.005$  | 8.193  | 8.193      | $8.189 \pm 0.004$  |
| $b$                                              | 8.144     | 8.144      | $8.152 \pm 0.005$  | 8.193  | 8.193      | $8.189 \pm 0.004$  |
| $c$                                              | 5.969     | 5.969      | $5.962 \pm 0.004$  | 5.973  | 5.973      | $5.976 \pm 0.004$  |
| tetragonal perovskite ( $I4/mcm$ , $a^0a^0c^-$ ) |           |            |                    |        |            |                    |
| $\Delta E$                                       | 4.4       | 3.7        | $4.0 \pm 0.4$      | 3.5    | 2.5        | $3.1 \pm 0.3$      |
| $a$                                              | 8.141     | 8.141      | $8.148 \pm 0.003$  | 8.188  | 8.188      | $8.185 \pm 0.003$  |
| $b$                                              | 8.141     | 8.141      | $8.148 \pm 0.003$  | 8.188  | 8.188      | $8.185 \pm 0.003$  |
| $c$                                              | 11.945    | 11.945     | $11.934 \pm 0.006$ | 11.951 | 11.951     | $11.959 \pm 0.009$ |
| cubic perovskite ( $Pm\bar{3}m$ , $a^0a^0a^0$ )  |           |            |                    |        |            |                    |
| $\Delta E$                                       | 17.3      | 17.8       | $17.9 \pm 0.5$     | 15.5   | 15.4       | $16.6 \pm 0.4$     |
| $a$                                              | 5.880     | 5.880      | $5.883 \pm 0.001$  | 5.896  | 5.896      | $5.899 \pm 0.001$  |
| $b$                                              | 5.880     | 5.880      | $5.883 \pm 0.001$  | 5.896  | 5.896      | $5.899 \pm 0.001$  |
| $c$                                              | 5.880     | 5.880      | $5.883 \pm 0.001$  | 5.896  | 5.896      | $5.899 \pm 0.001$  |
| $\delta$ -phase ( $Pnma$ )                       |           |            |                    |        |            |                    |
| $\Delta E$                                       | -13.0     | -12.3      | $-12.5 \pm 0.5$    | -4.1   | -4.2       | $-3.4 \pm 0.3$     |
| $a$                                              | 9.663     | 4.558      | $4.573 \pm 0.009$  | 4.606  | 4.614      | $4.597 \pm 0.007$  |
| $b$                                              | 4.558     | 9.663      | $9.606 \pm 0.020$  | 9.719  | 9.713      | $9.747 \pm 0.025$  |
| $c$                                              | 16.738    | 16.738     | $16.761 \pm 0.017$ | 16.875 | 16.886     | $16.885 \pm 0.030$ |

Table S4: Comparison (part 1) of energy differences  $\Delta E$  for CsPbI<sub>3</sub> structures relative to the orthorhombic phase in meV/atom and lattice parameters  $a$ ,  $b$ , and  $c$  in Å from density functional theory (DFT) calculations as well as the neuroevolution potential (NEP) models constructed in this work. For the latter results are given both for the models trained against the full set and model ensembles. In the latter case, the uncertainty obtained as the standard deviation across the models in the ensemble is given as well.

| CsPbI <sub>3</sub>                               | vdW-DF-cx |            |                    | SCAN   |            |                    |
|--------------------------------------------------|-----------|------------|--------------------|--------|------------|--------------------|
|                                                  | DFT       | NEP (full) | NEP (ensemble)     | DFT    | NEP (full) | NEP (ensemble)     |
| orthorhombic ( $Pnma$ , $a^-a^-c^+$ )            |           |            |                    |        |            |                    |
| $a$                                              | 8.166     | 8.172      | $8.192 \pm 0.028$  | 8.470  | 8.470      | $8.462 \pm 0.019$  |
| $b$                                              | 9.089     | 9.102      | $9.090 \pm 0.016$  | 9.059  | 9.059      | $9.068 \pm 0.016$  |
| $c$                                              | 12.451    | 12.455     | $12.465 \pm 0.008$ | 12.542 | 12.542     | $12.554 \pm 0.008$ |
| tetragonal perovskite ( $P4/mbm$ , $a^0a^0c^+$ ) |           |            |                    |        |            |                    |
| $\Delta E$                                       | 9.5       | 7.3        | $8.6 \pm 0.7$      | 7.3    | 5.4        | $6.2 \pm 0.3$      |
| $a$                                              | 8.622     | 8.622      | $8.628 \pm 0.003$  | 8.709  | 8.709      | $8.708 \pm 0.003$  |
| $b$                                              | 8.622     | 8.622      | $8.628 \pm 0.003$  | 8.709  | 8.709      | $8.708 \pm 0.003$  |
| $c$                                              | 6.369     | 6.369      | $6.366 \pm 0.003$  | 6.406  | 6.406      | $6.404 \pm 0.005$  |
| tetragonal perovskite ( $I4/mcm$ , $a^0a^0c^-$ ) |           |            |                    |        |            |                    |
| $\Delta E$                                       | 9.6       | 8.1        | $9.1 \pm 0.5$      | 7.3    | 5.7        | $6.5 \pm 0.3$      |
| $a$                                              | 8.620     | 8.620      | $8.626 \pm 0.002$  | 8.703  | 8.703      | $8.706 \pm 0.004$  |
| $b$                                              | 8.620     | 8.620      | $8.626 \pm 0.002$  | 8.703  | 8.703      | $8.706 \pm 0.004$  |
| $c$                                              | 12.734    | 12.734     | $12.727 \pm 0.007$ | 12.807 | 12.807     | $12.801 \pm 0.011$ |
| cubic perovskite ( $Pm\bar{3}m$ , $a^0a^0a^0$ )  |           |            |                    |        |            |                    |
| $\Delta E$                                       | 26.5      | 26.3       | $26.4 \pm 0.6$     | 22.7   | 20.9       | $21.5 \pm 0.3$     |
| $a$                                              | 6.267     | 6.260      | $6.261 \pm 0.002$  | 6.304  | 6.304      | $6.301 \pm 0.002$  |
| $b$                                              | 6.267     | 6.260      | $6.261 \pm 0.002$  | 6.304  | 6.304      | $6.301 \pm 0.002$  |
| $c$                                              | 6.267     | 6.260      | $6.261 \pm 0.002$  | 6.304  | 6.304      | $6.301 \pm 0.002$  |
| $\delta$ -phase ( $Pnma$ )                       |           |            |                    |        |            |                    |
| $\Delta E$                                       | -26.5     | -27.2      | $-26.5 \pm 0.4$    | -16.1  | -16.6      | $-15.9 \pm 0.2$    |
| $a$                                              | 4.786     | 4.786      | $4.768 \pm 0.015$  | 4.805  | 4.805      | $4.817 \pm 0.010$  |
| $b$                                              | 10.341    | 10.341     | $10.376 \pm 0.017$ | 10.616 | 10.624     | $10.601 \pm 0.029$ |
| $c$                                              | 17.664    | 17.664     | $17.710 \pm 0.042$ | 17.955 | 17.938     | $17.939 \pm 0.017$ |

Table S5: Comparison (part 2) of energy differences  $\Delta E$  for CsPbI<sub>3</sub> structures relative to the orthorhombic phase in meV/atom and lattice parameters  $a$ ,  $b$ , and  $c$  in Å from density functional theory (DFT) calculations as well as the neuroevolution potential (NEP) models constructed in this work. For the latter results are given both for the models trained against the full set and model ensembles. In the latter case, the uncertainty obtained as the standard deviation across the models in the ensemble is given as well.

| CsPbI <sub>3</sub>                               | PBEsol |            |                    | PBE    |            |                    |
|--------------------------------------------------|--------|------------|--------------------|--------|------------|--------------------|
|                                                  | DFT    | NEP (full) | NEP (ensemble)     | DFT    | NEP (full) | NEP (ensemble)     |
| orthorhombic ( $Pnma$ , $a^-a^-c^+$ )            |        |            |                    |        |            |                    |
| $a$                                              | 8.238  | 8.238      | $8.256 \pm 0.038$  | 8.632  | 8.632      | $8.644 \pm 0.018$  |
| $b$                                              | 9.029  | 9.029      | $9.020 \pm 0.023$  | 9.164  | 9.164      | $9.172 \pm 0.010$  |
| $c$                                              | 12.447 | 12.447     | $12.428 \pm 0.014$ | 12.666 | 12.666     | $12.661 \pm 0.006$ |
| tetragonal perovskite ( $P4/mbm$ , $a^0a^0c^+$ ) |        |            |                    |        |            |                    |
| $\Delta E$                                       | 7.7    | 7.1        | $6.8 \pm 0.5$      | 6.6    | 6.1        | $6.2 \pm 0.5$      |
| $a$                                              | 8.604  | 8.604      | $8.602 \pm 0.002$  | 8.830  | 8.830      | $8.830 \pm 0.006$  |
| $b$                                              | 8.604  | 8.604      | $8.602 \pm 0.002$  | 8.830  | 8.830      | $8.830 \pm 0.006$  |
| $c$                                              | 6.341  | 6.341      | $6.341 \pm 0.002$  | 6.474  | 6.474      | $6.477 \pm 0.003$  |
| tetragonal perovskite ( $I4/mcm$ , $a^0a^0c^-$ ) |        |            |                    |        |            |                    |
| $\Delta E$                                       | 7.9    | 7.2        | $7.0 \pm 0.4$      | 6.6    | 6.4        | $6.9 \pm 0.4$      |
| $a$                                              | 8.601  | 8.601      | $8.600 \pm 0.004$  | 8.832  | 8.832      | $8.832 \pm 0.006$  |
| $b$                                              | 8.601  | 8.601      | $8.600 \pm 0.004$  | 8.832  | 8.832      | $8.832 \pm 0.006$  |
| $c$                                              | 12.679 | 12.679     | $12.678 \pm 0.004$ | 12.947 | 12.947     | $12.949 \pm 0.009$ |
| cubic perovskite ( $Pm\bar{3}m$ , $a^0a^0a^0$ )  |        |            |                    |        |            |                    |
| $\Delta E$                                       | 25.4   | 25.8       | $25.5 \pm 0.7$     | 20.8   | 20.1       | $20.4 \pm 0.4$     |
| $a$                                              | 6.245  | 6.245      | $6.240 \pm 0.001$  | 6.386  | 6.386      | $6.386 \pm 0.001$  |
| $b$                                              | 6.245  | 6.245      | $6.240 \pm 0.001$  | 6.386  | 6.386      | $6.386 \pm 0.001$  |
| $c$                                              | 6.245  | 6.245      | $6.240 \pm 0.001$  | 6.386  | 6.386      | $6.386 \pm 0.001$  |
| $\delta$ -phase ( $Pnma$ )                       |        |            |                    |        |            |                    |
| $\Delta E$                                       | -15.6  | -14.8      | $-15.5 \pm 0.4$    | -9.9   | -10.2      | $-10.1 \pm 0.4$    |
| $a$                                              | 4.770  | 4.770      | $4.758 \pm 0.017$  | 4.880  | 4.880      | $4.877 \pm 0.014$  |
| $b$                                              | 10.366 | 10.366     | $10.405 \pm 0.029$ | 10.915 | 10.915     | $11.040 \pm 0.109$ |
| $c$                                              | 17.651 | 17.651     | $17.688 \pm 0.036$ | 18.169 | 18.169     | $18.087 \pm 0.075$ |

## Supplemental References

- [1] Zheyong Fan, Yanzhou Wang, Penghua Ying, Keke Song, Junjie Wang, Yong Wang, Zezhu Zeng, Ke Xu, Eric Lindgren, J. Magnus Rahm, Alexander J. Gabourie, Jiahui Liu, Haikuan Dong, Jianyang Wu, Yue Chen, Zheng Zhong, Jian Sun, Paul Erhart, Yanjing Su, and Tapio Ala-Nissila. GPUMD: A package for constructing accurate machine-learned potentials and performing highly efficient atomistic simulations. *Journal of Chemical Physics*, 157:114801, 2022. doi: 10.1063/5.0106617.
- [2] Ryosuke Jinnouchi, Jonathan Lahnsteiner, Ferenc Karsai, Georg Kresse, and Menno Bokdam. Phase transitions of hybrid perovskites simulated by machine-learning force fields trained on the fly with Bayesian inference. *Physical Review Letters*, 122:225701, 2019. doi: 10.1103/PhysRevLett.122.225701.
- [3] Jonathan Lahnsteiner and Menno Bokdam. Anharmonic lattice dynamics in large thermodynamic ensembles with machine-learning force fields: CsPbBr<sub>3</sub> a phonon liquid with Cs rattlers. *Physical Review B*, 105:024302, 2022. doi: 10.1103/PhysRevB.105.024302.
